# Supplementary material for: Solvation Restructuring Accelerates Early SEI Nucleation in Lithium Metal Batteries
Source: arXiv:2602.05141 source file (2026-08-14)
Supplement: Supplementary file 1 [file SI.pdf]

# Supporting Information

# Predictive Machine Learning Molecular Dynamics of SEI Formation in Concentrated LiTFSI and $LiPF_6$ Electrolytes for Lithium Metal Batteries

*Syed Mustafa Shah* [a,+], *Mohammed Lemaalem* [a,+], *Anh T. Ngo* [a,b,*]

[a] Department of Chemical Engineering, University of Illinois Chicago, Chicago, IL 60608, USA

[b] Materials Science Division, Argonne National Laboratory, Lemont, IL 60439, USA.

[+] These authors contributed equally to this work.

*(*) anhngo@uic.edu*

## Table of Contents

### Supplementary Texts

- **Section S1:** AIMD simulation details
- **Section S2:** Deep Potential methodology and hyperparameters
- **Section S3:** Deep Potential validation
- **Section S4:** Machine learning molecular dynamics simulations
- **Section S5:** Classical molecular dynamics simulation details
- **Section S6:** Structural properties calculation
- **Section S7:** Dynamics properties calculation
- **Section S8:** MLMD investigation of Li-metal anode/electrolyte interfacial structure

### Supplementary Figures

- **Figure S1:** Parity plots for 1.5 M LiTFSI electrolyte
- **Figure S2:** Parity plots for 2.5 M LiTFSI electrolyte
- **Figure S3:** Parity plots for 3.5 M LiTFSI electrolyte
- **Figure S4:** Parity plots for 1 M $LiPF_6$ electrolyte
- **Figure S5:** Parity plots for LiTFSI electrolytes/Li metal interface
- **Figure S6:** Parity plots for 1 M $LiPF_6$ electrolyte/Li metal interface

- **Figure S7:** Ion transport (MSD) and MLMD snapshots
- **Figure S8:** Time-dependent structural evolution at LiTFSI/Li interface


**Supplementary Tables**


- **Table S1:** AIMD simulation cell parameters and densities
- **Table S2:** Molecular compositions of electrolyte systems
- **Table S3:** MLMD simulation cell parameters and densities
- **Table S4:** CMD Simulation Parameters
- **Table S5:** Interface simulation cell parameters

# S1 AIMD simulation detail

The number of solute molecules ($N_{\text{solute}}$) for LiTFSI and $LiPF_6$ was calculated directly from the target molar concentration ($C_{\text{molar}}$), as described in Equation S1. For instance, achieving a concentration of 1.5 M LiTFSI within the defined simulation volume required the insertion of approximately 2 LiTFSI molecules.

$$N_{\text{solute}} = C_{\text{molar}} \times V_{\text{box}} \times N_A \tag{S1}$$

Conversely, the number of solvent molecules ($N_{\text{solvent}}$) for DMC, EMC, and EC was derived using a density-based approach to ensure that the system approximated experimental bulk densities. This was calculated by determining the total mass of solvent required to fill the volume ($V_{\text{box}}$) based on its density ($\rho$), and then converting this mass to the number of molecules using the molar mass ($M_w$), as shown in Equation S2.

$$N_{\text{solvent}} = \left( \frac{\rho \times V_{\text{box}}}{M_w} \right) \times N_A \tag{S2}$$

Here, $N_A$ represents Avogadro's constant ($6.022 \times 10^{23}$ mol$^{-1}$).
Initial atomic configurations were generated using the PACKMOL package [1], reflecting experimental compositions (Table S2 and Table S1). Classical MD simulations were performed to optimize the initial structures of four electrolyte systems: 1.5 M, 2.5 M, and 3.5 M LiTFSI/DMC, and 1 M $LiPF_6$/DMC:EC:EMC (1:1:1) for subsequent AIMD simulations. These classical MD runs served to remove any overlapping atoms or structural misarrangements generated by the PACKMOL packing algorithm, ensuring high-quality initial geometries. All simulations were conducted using LAMMPS [2] with the OPLS-AA force field [3, 4, 5]. The optimization protocol included energy minimization followed by equilibration at 300 K and 1 bar to match experimental conditions. Once converged structures were obtained, they were used as input for the AIMD calculations. For the AIMD simulation, the Perdew–Burke–Ernzerhof (PBE) functional within the Generalized Gradient Approximation (GGA) [6] was used to describe the exchange–correlation energy. A plane-wave basis set with a cutoff energy of 550 eV was applied to ensure convergence. Core–valence interactions were treated using the projector augmented wave (PAW) method [7, 8]. The Brillouin zone was sampled at the Gamma point using a $4 \times 4 \times 4$ k-mesh [9]. Energy convergence criteria were set at $1 \times 10^{-5}$ eV for K-point integration, and structural optimization was performed until the forces on each atom were below 0.001 eV/Å.

Table S1: AIMD simulation cell parameters and densities.

| **System** | **Atoms** | $\mathbf{L_x}$ (Å) | $\mathbf{L_y}$ (Å) | $\mathbf{L_z}$ (Å) | **Cell volume** (Å$^3$) | **Density** (g cm$^{-3}$) |
|---|---|---|---|---|---|---|
| 1.5 M LiTFSI | 224 | 13.53 | 13.53 | 13.53 | 2477 | 1.35 |
| 2.5 M LiTFSI | 240 | 13.81 | 13.81 | 13.81 | 2634 | 1.45 |
| 3.5 M LiTFSI | 272 | 14.55 | 14.55 | 14.55 | 3080 | 1.55 |
| 1 M $LiPF_6$ | 317 | 15.16 | 15.17 | 15.14 | 3482 | 1.26 |

The optimized simulation cells were subjected to *ab initio* molecular dynamics (AIMD) simulations at 300 K in the canonical (NVT) ensemble to generate training datasets for the Deep Potential (DP) model. AIMD simulations were performed with a time step of `POTIM` = 1 fs for approximately 4 ps. To obtain a more refined sampling of fast hydrogen dynamics, an additional AIMD trajectory was carried out with a reduced time step of `POTIM` = 0.5 fs for about 2 ps, ensuring improved resolution of high-frequency vibrational modes.

To further enrich the diversity and transferability of the dataset and to ensure the model accurately captures bond-breaking events during SEI nucleation, additional AIMD simulations were conducted at elevated temperatures of 700 K, 1200 K, and 1500 K, each for approximately 4 ps. These conditions naturally induced molecular fragmentation and radical formation, populating the dataset with relevant decomposition intermediates (e.g., TFSI radicals, solvent fragments) necessary for learning the reactive potential energy surface. Furthermore, simulations involving unit-cell compression (0.7) and expansion (1.2) were performed for about 2 ps each, enabling sampling under varying volumetric conditions. All AIMD trajectories generated under different temperatures, time steps, and cell deformations were combined into a single, comprehensive dataset, which was subsequently used for training the DP. This diverse dataset ensured that the resulting model is both accurate and highly transferable across a wide range of thermodynamic and structural environments.

# S2 Deep Potential methodology and hyperparameters

## S2.1 Mathematical framework of the `se_e2_a` descriptor

In the DeepPot-SE framework used in this work, the local atomic environment around atom $i$ is represented by the two-body embedding smooth edition (`se_e2_a`) descriptor. The descriptor $\mathcal{D}^i \in \mathbb{R}^{M \times M_<}$ is constructed from the neighbor list of atom $i$, considering a maximum of $N_c$ neighbors within the cutoff radius $r_c$.

The coordinate matrix $\mathcal{R}^i \in \mathbb{R}^{N_c \times 4}$ is defined as:

$$(\mathcal{R}^i)_j = \left( s(r_{ij}),\ \frac{s(r_{ij})\, x_{ij}}{r_{ij}},\ \frac{s(r_{ij})\, y_{ij}}{r_{ij}},\ \frac{s(r_{ij})\, z_{ij}}{r_{ij}} \right), \tag{S3}$$

where $\boldsymbol{r}_{ij} = \boldsymbol{r}_j - \boldsymbol{r}_i = (x_{ij}, y_{ij}, z_{ij})$ is the relative coordinate of neighbor $j$ with respect to atom $i$, and $r_{ij} = \|\boldsymbol{r}_{ij}\|$.

To ensure smoothness, a switching function $s(r)$ is applied:

$$s(r) = \begin{cases} \frac{1}{r}, & r < r_s, \\ \frac{1}{r}\left[x^3(-6x^2 + 15x - 10) + 1\right], & r_s \le r < r_c, \\ 0, & r \ge r_c, \end{cases} \tag{S4}$$

where $x = (r - r_s)/(r_c - r_s)$. This form ensures that $s(r)$ is smooth (up to the second derivative) in the interval $[r_s, r_c)$ and decays to zero at the cutoff. In our simulations, we used a cutoff radius $r_c = 6.00$ Å and a smoothing start radius $r_s = 0.50$ Å.

Table S2: Molecular compositions of electrolyte systems used in AIMD, MLMD, CMD, and interface simulations. All counts are given as numbers of molecules, except Li, which is given as number of atoms.

| **Simulation** | **System** | **LiTFSI** | **$LiPF_6$** | **DMC** | **EMC** | **EC** | |
|---|---|---|---|---|---|---|---|
| AIMD | 1.5 M LiTFSI | 2 | – | 16 | – | – | |
| | 2.5 M LiTFSI | 3 | – | 16 | – | – | |
| | 3.5 M LiTFSI | 5 | – | 16 | – | – | |
| | 1.0 M $LiPF_6$ | – | 4 | 8 | 7 | 10 | |
| MLMD | 1.5 M LiTFSI | 128 | – | 1024 | – | – | |
| | 2.5 M LiTFSI | 192 | – | 1024 | – | – | |
| | 3.5 M LiTFSI | 320 | – | 1024 | – | – | |
| | 1.0 M $LiPF_6$ | – | 128 | 512 | 448 | 640 | |
| CMD | 1.5 M LiTFSI | 800 | – | 6400 | – | – | |
| | 2.5 M LiTFSI | 1224 | – | 6400 | – | – | |
| | 3.5 M LiTFSI | 1995 | – | 6400 | – | – | |
| | 1.0 M $LiPF_6$ | – | 788 | 3152 | 2758 | 3940 | |
| | | **LiTFSI** | **$LiPF_6$** | **DMC** | **EMC** | EC | **Li** |
| Interface | 1.5M LiTFSI/Li | 64 | - | 512 | - | - | 3328 |
| | 2.5M LiTFSI/Li | 96 | - | 512 | - | - | 3328 |
| | 3.5M LiTFSI/Li | 160 | - | 512 | - | - | 3328 |
| | 1.0M $LiPF_6$/Li | - | 64 | 256 | 224 | 320 | 3328 |

The embedding matrix $\mathcal{G}^i \in \mathbb{R}^{N_c \times M}$ is computed by a fully connected neural network $\mathcal{N}_{e,2}$ applied to the switching function values:

$$(\mathcal{G}^i)_j = \mathcal{N}_{e,2}\big(s(r_{ij})\big). \tag{S5}$$

The reduced embedding matrix $\mathcal{G}^i_< \in \mathbb{R}^{N_c \times M_<}$ retains only the first $M_<$ columns of $\mathcal{G}^i$. The final descriptor is then given by:

$$\mathcal{D}^i = \frac{1}{N_c^2}(\mathcal{G}^i)^T \mathcal{R}^i (\mathcal{R}^i)^T \mathcal{G}^i_<. \tag{S6}$$

## S2.2 Model architecture and hyperparameters

For the descriptor setup, the maximum number of neighbors (`sel`) was set based on the system composition. For the varying concentration systems ([H, Li, C, N, O, F, S]), `sel` was set to [77, 2, 42, 2, 45, 10, 4], resulting in an effective $N_c = 77$. For the 1M $LiPF_6$ system ([H, Li, C, O, F, P]), `sel` was set to [115, 2, 66, 60, 10, 2], resulting in $N_c = 115$.

The embedding network $\mathcal{N}_{e,2}$ utilized an architecture of $[25, 50, 1]$, yielding an embedding dimension $M = 100$ with a reduced dimension $M_< = 16$. The descriptor was constructed with `type_one_side:true` (the embedding network depends only on the neighbor type)

and `resnet_dt:false`. The fitting network, which maps the descriptor to atomic energies, consisted of three fully connected layers with 200 neurons each. Residual connections (`resnet_dt= true`) were enabled to improve stability and convergence.

### S2.3 Training protocol

Training was performed for $1{\times}10^6$ steps using separate training and validation datasets, with fixed random seeds to ensure reproducibility. An exponential learning rate schedule was used, decreasing from an initial rate of $1{\times}10^{-3}$ to a final rate of $3.5{\times}10^{-8}$, with a decay step of 5000.

The total loss function $L$ combined errors from energy ($L_e$), forces ($L_f$), and virials ($L_v$) using adaptive dimensionless prefactors ($p_e, p_f, p_v$):

$$L = p_e L_e + p_f L_f + p_v L_v \tag{S7}$$

These prefactors were adjusted during training according to the learning rate. The energy weight ($p_e$) increased from 0.02 to 1, the force weight ($p_f$) decreased from 1000 to 1, and the virial weight ($p_v$) increased from 0.02 to 1.

## S3 Deep Potential validation

The interatomic potential was constructed using the Deep Potential Smooth Edition (DeepPot-SE) formalism. The local atomic environment around each atom is represented by the two-body embedding descriptor (se_e2_a) with a cutoff radius set to $r_c$ = 6.00 Å. This descriptor ensures continuity up to the second derivative, guaranteeing smooth energy and force predictions necessary for stable molecular dynamics.

The potential energy surface was fitted using a fully connected neural network trained on the generated AIMD datasets. The training process minimized a composite loss function that included weighted errors for energies, forces, and virials. An adaptive weighting scheme was employed, emphasizing force accuracy during early training stages and gradually balancing energy and virial contributions as convergence approached.

The resulting Deep Potential exhibits excellent fidelity against the AIMD ground truth. As shown in Figures S1-S6, training and validation Root Mean Square Error (RMSE) curves converge rapidly without overfitting across all simulated electrolyte systems. The accuracy is further corroborated by energy parity plots (see Main paper Figure 1(B) and Figures S5 and S6), demonstrating a near-perfect linear correlation ($R^2 = 0.99$). Crucially, element-wise force predictions show high consistency with AIMD forces, yielding coefficients of determination ($R^2$) ranging from 0.96 to 0.99 for all constituent species (Figures S1-S6).

## S4 Machine learning molecular dynamics simulations

Machine learning molecular dynamics (MLMD) simulations were conducted in the NVT ensemble using the LAMMPS simulation package [2] coupled with the DeepMD-kit [10, 11]. The MLMD simulations utilized the same initial structures and thermodynamic conditions

as the reference AIMD simulations. The structural fidelity of the generated Deep Potential model was assessed by comparing atomic trajectories from AIMD and MLMD at 298 K using Radial Distribution Functions (RDFs). Because RDFs are sensitive measures of short-range order and interatomic correlations, their agreement serves as a robust confirmation of the potential's reliability. Figure 1(C) in the main paper presents the site-site RDFs for Li–N, Li–O, Li–F, and Li–P pairs across varying concentrations of LiTFSI (1.5 M, 2.5 M, and 3.5 M) and for the 1 M $LiPF_6$ system. In all investigated systems, the MLMD profiles (dashed lines) exhibit a remarkable overlap with the AIMD results (solid lines), successfully reproducing specific structural features across different concentrations. In the lower concentration LiTFSI systems, lithium is primarily coordinated by oxygen. For 1.5 M LiTFSI, the Li–O RDF shows a sharp primary peak at 2.1 Å and a secondary structure around 4 Å; at 2.5 M, the primary Li–O peak is located at 2.3 Å. Due to steric shielding by the bulky sulfonyl groups in the $TFSI^-$ anion, direct Li–N coordination is absent in these lower concentrations, with the first Li–N peak appearing distantly at 4.25 Å for 1.5 M and 3.65 Å for 2.5 M. Similarly, Li–F interactions manifest as broad, hollow peaks centered far from the cation (e.g., 6.75 Å at 1.5 M and 4.5 Å at 2.5 M). As the concentration increases to 3.5 M LiTFSI, a significant structural shift occurs due to solvent scarcity. While a primary Li–O peak remains at 2.1 Å (with a small secondary peak at 4 Å), anions are forced closer to cations. This results in the emergence of distinct short-range peaks for Li–N at 2.5 Å and Li–F at 2.65 Å, indicating increased contact ion pairing. The 1 M $LiPF_6$ system displays different solvation characteristics, showing sharp, co-located peaks for both Li–O and Li–F at approximately 2.25 Å. This signifies strong direct interaction with both solvent oxygen and anion fluorine atoms, while the central phosphorus remains distant at 3.6 Å. The ability of MLMD to precisely replicate these complex, concentration-dependent structural features observed in AIMD provides high confidence in the model's fidelity. However, while AIMD provides an accurate ground truth for these specific structures, the small number of particles feasible in AIMD simulations is insufficient for efficiently evaluating the macroscopic structure and long-range correlations characteristic of real electrolytes. To overcome these finite-size limitations and obtain robust statistical properties, the investigation was extended by utilizing the validated Deep Potential to drive large-scale MLMD simulations. These larger systems were generated by replicating the small AIMD simulation boxes $4 \times 4 \times 4$ times along the Cartesian axes while strictly maintaining the experimental density, as summarized in Table S2 and Table S3. These large-scale simulations enable a comprehensive analysis unattainable with smaller simulation boxes.

Table S3: MLMD simulation cell parameters and densities.

| **System** | **Atoms** | $L_x$ (Å) | $L_y$ (Å) | $L_z$ (Å) | **Simulation cell** (Å$^3$) | **Density** (g cm$^{-3}$) |
|---|---|---|---|---|---|---|
| 1.5 M LiTFSI | 14336 | 54.12 | 54.12 | 54.12 | 158516 | 1.35 |
| 2.5 M LiTFSI | 15360 | 55.24 | 55.24 | 55.24 | 168563 | 1.45 |
| 3.5 M LiTFSI | 17408 | 58.20 | 58.20 | 58.20 | 197137 | 1.55 |
| 1 M $LiPF_6$ | 20288 | 60.64 | 60.64 | 60.64 | 222839 | 1.26 |

# S5 Classical molecular dynamics simulation detail

Classical molecular dynamics (CMD) simulations were performed using LAMMPS [12] for LiTFSI/DMC (1.5–3.5 M) and $LiPF_6$/DMC:EMC:EC (1 M) electrolytes (Table S2). OPLS–AA force-field parameters [3, 4, 5] were used for all species. A cutoff distance of $r_{\text{cut}} = 12$ Å was employed for both Lennard-Jones and short-range Coulombic interactions, with a time step of $\delta t = 1$ fs. Long-range electrostatics were treated using the particle–particle particle–mesh (PPPM) Ewald method with an accuracy of $10^{-4}$ [13, 14]. Initial configurations were generated using Moltemplate [15] in oversized simulation boxes to prevent atomic overlaps. Each system was compressed and equilibrated using the following NPT protocol: (1) Langevin dynamics at $T = 900$ K for 1 ns; (2) NPT equilibration using the Nosé–Hoover thermostat at 900 K; (3) compression at 100 bar; (4) relaxation from 100 bar to 1 bar; and (5) final equilibration at $T = 300$ K and $P = 1$ bar for 5 ns. Table S4 summarizes the resulting system compositions and simulation box geometries. The Production runs for structural and transport property analysis were carried out in the NVT ensemble at 300 K using the Nosé–Hoover thermostat.

Table S4: CMD Simulation Parameter.

| System | Atoms | $L_x$ (Å) | $L_y$ (Å) | $L_z$ (Å) | Simulation cell (Å$^3$) | Density (g cm$^{-3}$) |
|---|---|---|---|---|---|---|
| 1.5 M LiTFSI | 89600 | 104 | 104 | 104 | 1124960 | 1.19 |
| 2.5 M LiTFSI | 97920 | 104.94 | 104.94 | 104.94 | 1155540 | 1.35 |
| 3.5 M LiTFSI | 106352 | 108.56 | 108.56 | 108.56 | 1279300 | 1.46 |
| 1 M $LiPF_6$ | 124898 | 114.10 | 114.10 | 114.10 | 1485464 | 1.16 |

# S6 Structural properties calculation

The structural properties employed the coordination number $N(r)$ and Radial Distribution Function $g(r)$ to analyze how particles are distributed in space and how local structures form in the electrolyte. The pair distribution function $g_{\alpha\beta}(r)$ is defined as:

$$g_{\alpha\beta}(r) = \frac{\langle \rho_\beta(r) \rangle}{\langle \rho_\beta \rangle_{\text{local}}} = \frac{1}{\langle \rho_\beta \rangle_{\text{local}}} \frac{1}{N_\alpha} \sum_{i\in\alpha}^{N_\alpha} \sum_{j\in\beta}^{N_\beta} \frac{\delta(r_{ij} - r)}{4\pi r^2} \tag{S8}$$

In this expression, $\langle \rho_\beta(r) \rangle$ represents the average number density of particles of type $\beta$ at a distance $r$ from particles of type $\alpha$, while $\langle \rho_\beta \rangle_{\text{local}}$ denotes the local average number density of $\beta$ particles computed over all spherical shells of radius $r_{\max}$ centered around $\alpha$ particles. In the present study, we set $r_{\max} = 12$ Å.

The coordination number, $N(r)$, refers to the count of neighboring particles located within a prescribed cutoff distance determined by the pair interaction potential from a given central particle. It can be calculated as:

$$N(r) = 2\pi \int_0^{r_c} n(r)\, r\, dr = 2\pi n_b \int_0^{r_c} g(r)\, r\, dr \tag{S9}$$

where $r_c$ is the cutoff radius, $n(r)$ is the local number density as a function of distance $r$, $n_b$ is the bulk number density, and $g(r)$ is the radial distribution function describing the probability of finding a particle at a distance $r$ from the reference particle.

# S7 Dynamics properties calculation

## S7.1 Ionic conductivity calculation

We characterized ion transport in the investigated electrolytes through the evaluation of Onsager transport coefficients. These coefficients, denoted as $L^{ij}$, offer a detailed physical interpretation of ion–ion correlations and can be obtained from molecular dynamics simulations via Green–Kubo (GK) relations. Our main objective is to quantify the dynamic behavior of the electrolytes, specifically the ionic conductivities of LiTFSI- and $LiPF_6$-based systems, using both classical molecular dynamics (CMD) and machine learning molecular dynamics (MLMD), and to benchmark these results against available experimental measurements.

Within the Green–Kubo formalism, the ionic conductivity $\sigma^{\mathrm{G-K}}$ is calculated from the time correlation of the total ionic current $\mathbf{J}$ in the system:

$$\sigma^{\mathrm{G-K}} = \frac{V}{k_{\mathrm{B}}T} \int_0^{\infty} dt \, \langle \mathbf{J}(t) \cdot \mathbf{J}(0) \rangle \tag{S10}$$

$$\mathbf{J}(t) = q \sum_{i=1}^{N} z_i \mathbf{v}_i(t) \tag{S11}$$

Here, $q$ denotes the elementary charge, $z_i$ is the valence of ion $i$, $\mathbf{v}_i(t)$ is its velocity, $T$ is the system temperature, $k_{\mathrm{B}}$ is the Boltzmann constant, $V$ is the simulation cell volume, and $N$ is the total number of ions.

The Green–Kubo relations may also be recast in terms of particle displacements rather than velocities. This formulation, conceptually similar to computing self-diffusion coefficients from mean-squared displacements (MSD), enables the evaluation of $L^{ij}$ coefficients directly from particle trajectories [16]:

$$L^{ij} = \frac{q^2}{6k_{\mathrm{B}}TV} \lim_{t\to\infty} \frac{d}{dt} \Big\langle \sum_{\alpha} [\boldsymbol{r}_i^{\alpha}(t) - \boldsymbol{r}_i^{\alpha}(0)] \cdot \sum_{\beta} [\boldsymbol{r}_j^{\beta}(t) - \boldsymbol{r}_j^{\beta}(0)] \Big\rangle \tag{S12}$$

where $\boldsymbol{r}_i^{\alpha}$ represents the position of particle $\alpha$ of species $i$, measured relative to the system's center of mass, and $k_{\mathrm{B}}T$ is the thermal energy.

The diagonal Onsager coefficients $L^{ii}$ can be decomposed into self and distinct contributions. The self-component is given by:

$$L^{ii}_{\mathrm{self}} = \frac{q^2}{6k_{\mathrm{B}}TV} \lim_{t\to\infty} \frac{d}{dt} \sum_{\alpha} \left\langle [\boldsymbol{r}_i^{\alpha}(t) - \boldsymbol{r}_i^{\alpha}(0)]^2 \right\rangle \tag{S13}$$

The distinct contribution follows from $L^{ii}_{\text{distinct}} = L^{ii} - L^{ii}_{\text{self}}$. The self-terms are directly linked to the self-diffusion coefficients $D_i$ through $L^{ii}_{\text{self}} = \frac{D_i c_i}{k_B T}$, where $c_i$ denotes the concentration of species $i$.

Assuming both ionic species are monovalent, the total ionic conductivity can be expressed as:

$$\sigma^{\text{G-K}} = L^{++} + L^{--} - 2L^{+-} \tag{S14}$$

### S7.2 Viscosity calculation

To quantify the internal friction resulting from molecular motion within LiTFSI- and $LiPF_6$-based electrolytes, viscosity was calculated using the Green–Kubo method. This approach involves integrating the autocorrelation function of the off-diagonal components of the pressure tensor:

$$\eta_{\alpha\beta} = \frac{V}{k_B T} \int_0^\infty \langle P_{\alpha\beta}(t_0) P_{\alpha\beta}(t_0 + t) \rangle_{t_0} \, dt \tag{S15}$$

where $P_{\alpha\beta}$ represents an off-diagonal element of the pressure tensor, with $\alpha, \beta = x, y, z$. The brackets $\langle \cdot \rangle_{t_0}$ denote averaging over multiple time origins $t_0$. To enhance statistical reliability, all off-diagonal pressure tensor components were incorporated into the calculation.

## S8 MLMD investigation of Li-metal anode/electrolyte interfacial structure

To establish a robust framework for studying electrolyte/anode interfaces, we first built interface models that couple a Li metal slab of thickness 20 Å with each of the four AIMD-optimized electrolyte systems (Table S2 and Table S5). The electrolytes training sets were then augmented with small-scale electrolyte–anode AIMD simulations at 300 K and used to retrain the model, explicitly incorporating the Li metal structure. The resulting validated Deep Potential is applied to simulate interfacial interactions (Figures S5 and S6), enabling a detailed investigation of the underlying interfacial mechanisms.

To quantify the extent of interfacial reactions, we evaluated time-resolved bond populations. A chemical bond was considered to form when the interatomic distance between a given pair of species fell below a species-specific cutoff radius, defined by the position of the first maximum in the corresponding radial distribution function. For the LiTFSI systems, the cutoff distances were set to 2.0 Å for Li–O, 2.1 Å for Li–F, 2.0 Å for Li–N, and 2.7 Å for Li–S. For the $LiPF_6$ system, the cutoff distances were 2.2 Å for Li–O, 2.0 Å for Li–F, and 3.5 Å for Li–P.

Table S5: Interface simulation cell parameters

| System | Atoms | $L_x$ (Å) | $L_y$ (Å) | $L_z$ (Å) | Cell volume ($Å^3$) |
|---|---|---|---|---|---|
| 1.5 M LiTFSI | 10496 | 52.64 | 52.38 | 62.49 | 172302.62 |
| 2.5 M LiTFSI | 11008 | 52.42 | 52.55 | 62.54 | 172277.12 |
| 3.5 M LiTFSI | 12864 | 62.86 | 63.83 | 63.84 | 256209.10 |
| 1 M $LiPF_6$ | 14272 | 61.08 | 60.96 | 66.11 | 246156.40 |

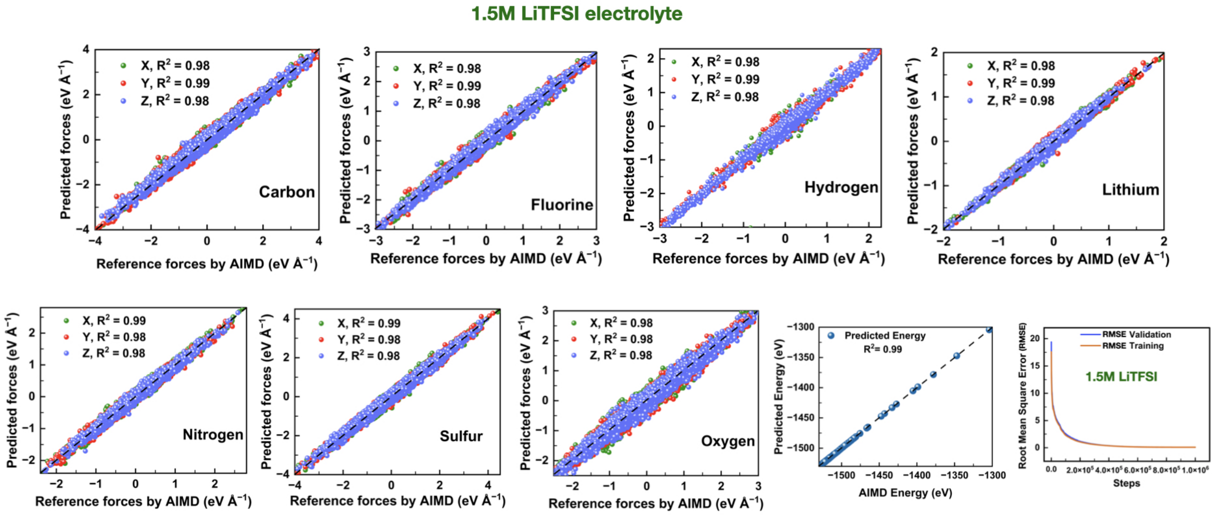


Figure S1: Parity plots comparing AIMD-calculated versus DP-predicted forces and energies for test configurations of 1.5 M LiTFSI electrolyte and the root-mean-square errors (RMSE) demonstrating high fidelity of the Deep Potential.

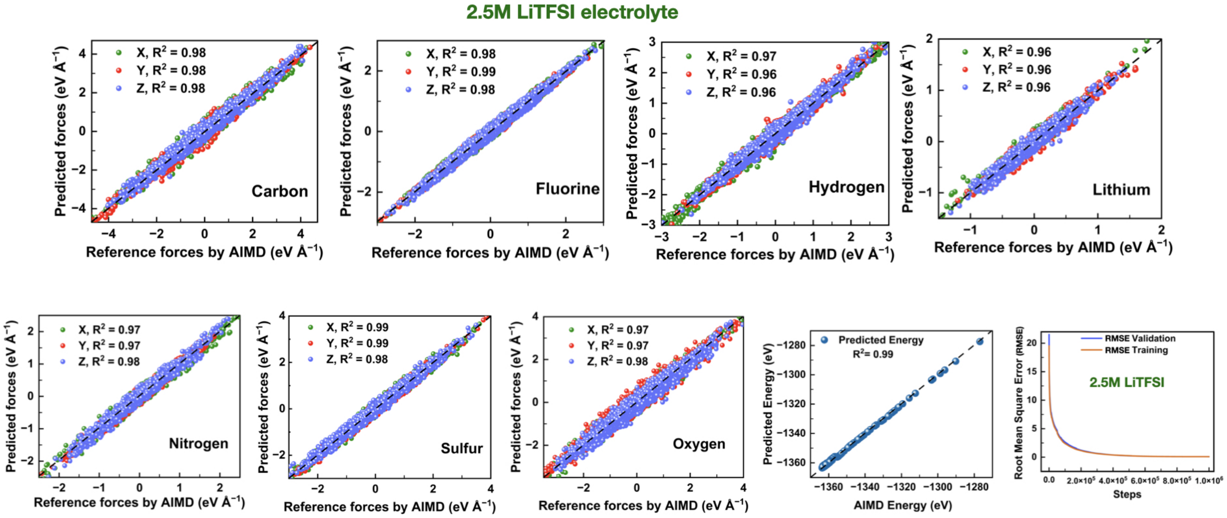


Figure S2: Parity plots comparing AIMD-calculated versus DP-predicted forces and energies for test configurations of 2.5 M LiTFSI electrolyte and the root-mean-square errors (RMSE) demonstrating high fidelity of the Deep Potential.

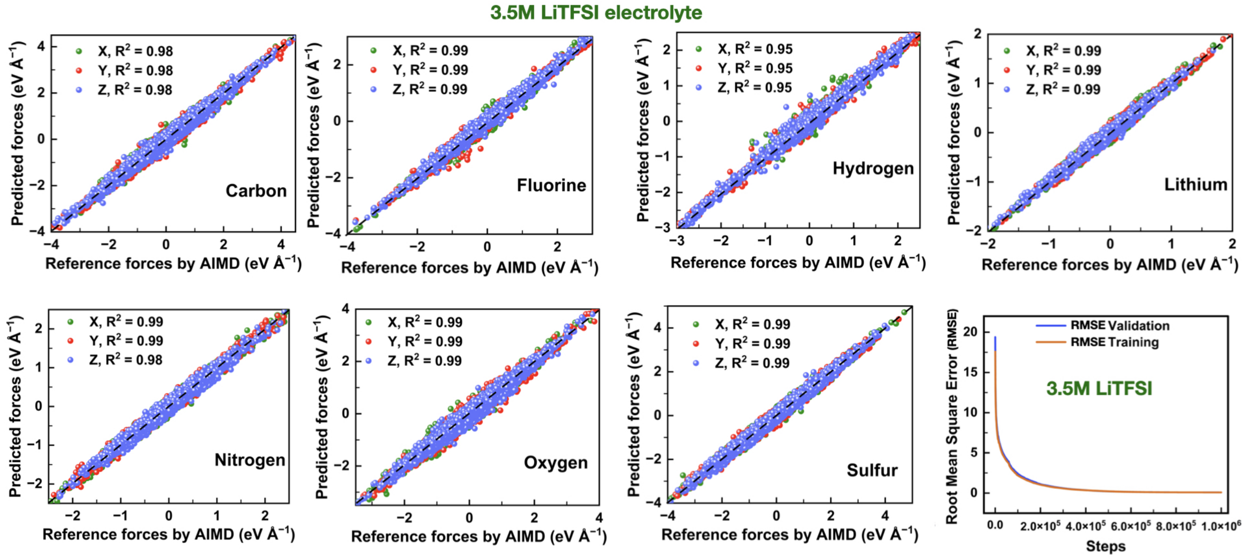


Figure S3: Parity plots comparing AIMD-calculated versus DP-predicted forces for test configurations of 3.5 M LiTFSI electrolyte and the root-mean-square errors (RMSE) demonstrating high fidelity of the Deep Potential.

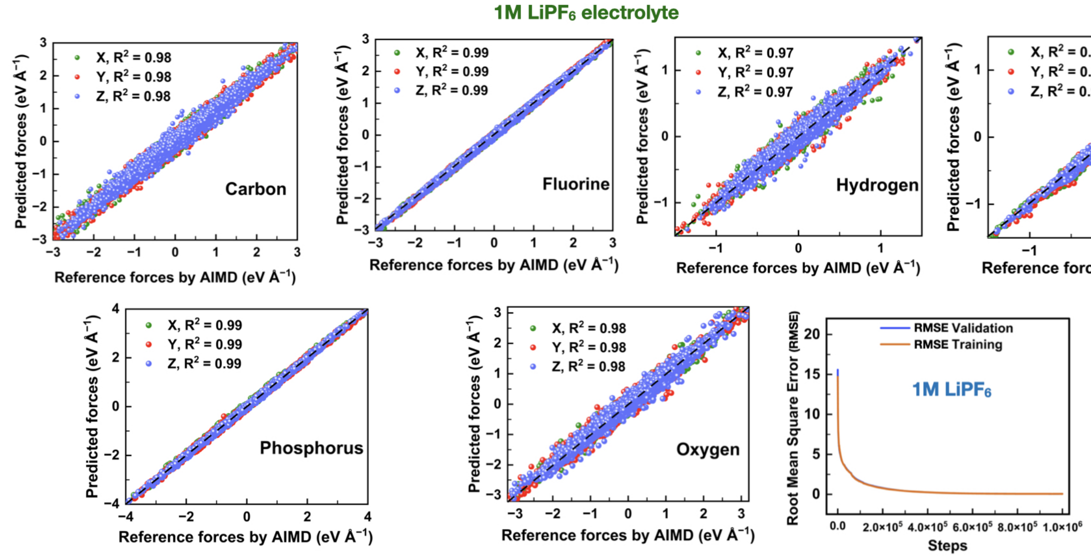


Figure S4: Parity plots comparing AIMD-calculated versus DP-predicted forces for test configurations of 1 M $LiPF_6$ electrolyte and the root-mean-square errors (RMSE) demonstrating high fidelity of the Deep Potential.

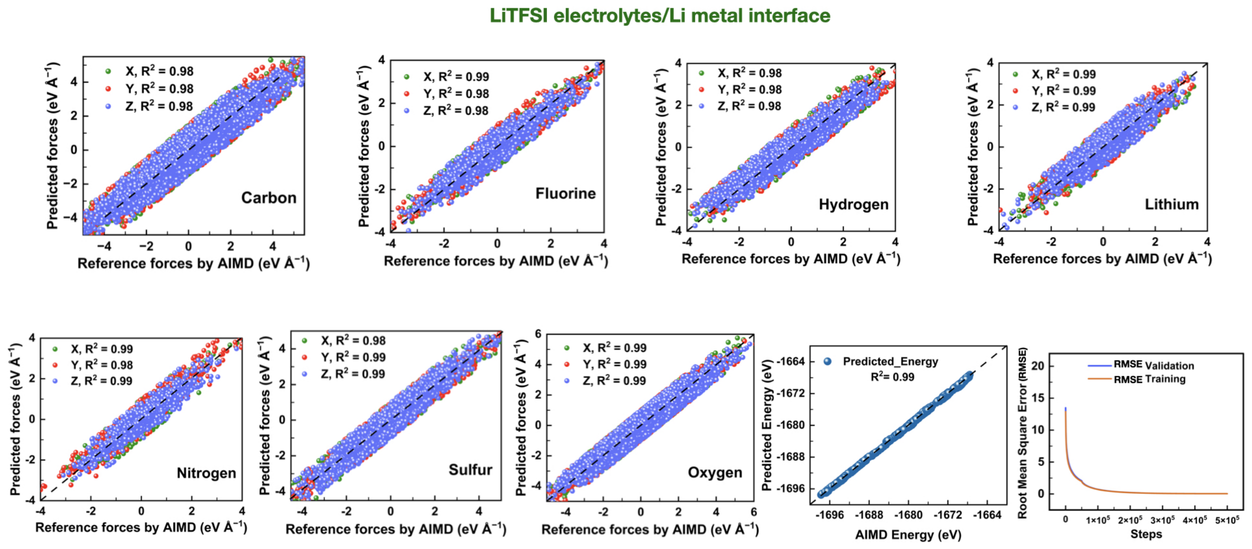


Figure S5: Parity plots comparing AIMD-calculated versus DP-predicted forces and energies for test configurations of LiTFSI electrolytes/Li metal interface and the root-mean-square errors (RMSE) demonstrating high fidelity of the Deep Potential.

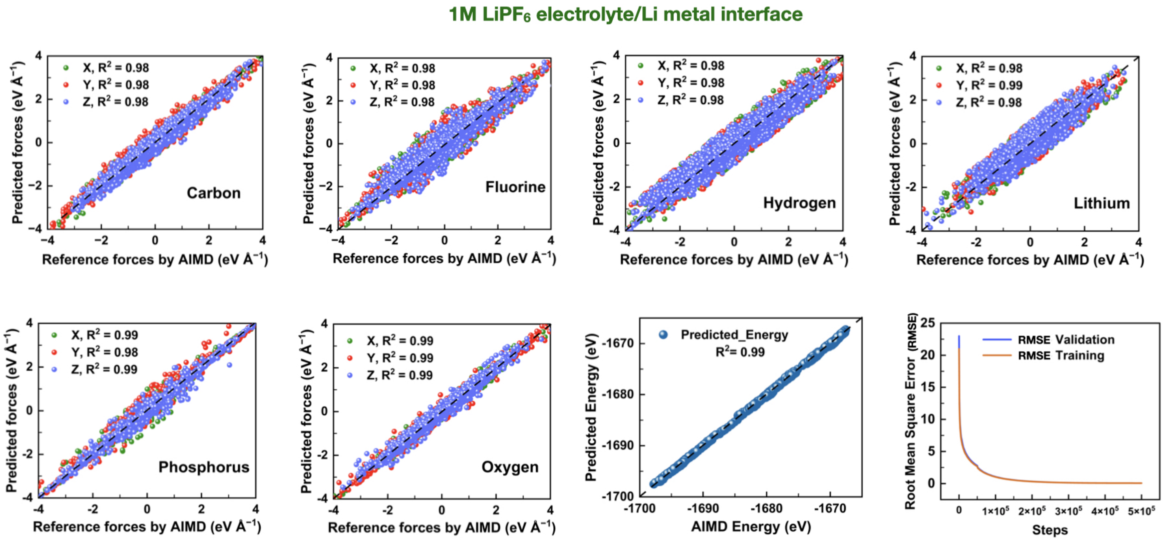


Figure S6: Parity plots comparing AIMD-calculated versus DP-predicted forces and energies for test configurations of 1 M $LiPF_6$ electrolyte/Li metal interface and the root-mean-square errors (RMSE) demonstrating high fidelity of the Deep Potential.

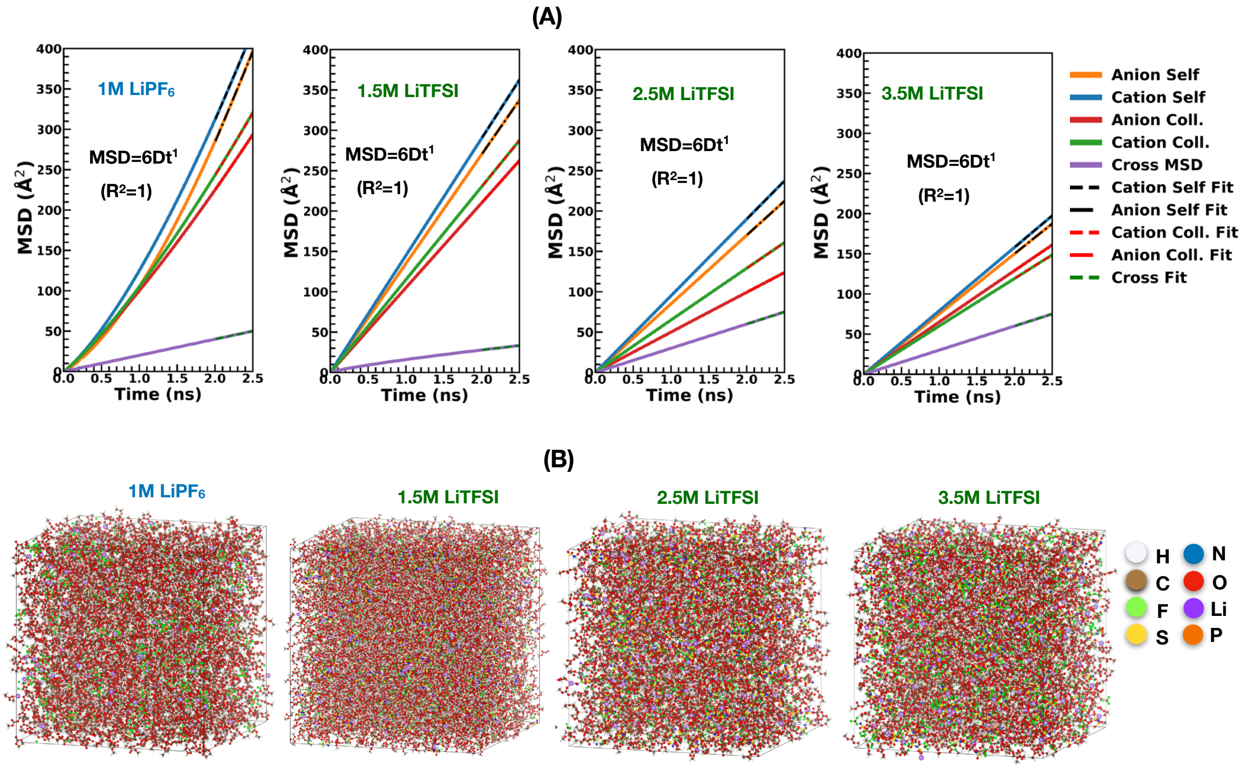


Figure S7: Ion transport from machine learning molecular dynamics: (A) mean square displacement of LiTFSI and $LiPF_6$ electrolytes at varying salt concentrations and (B) corresponding MLMD simulation snapshots.

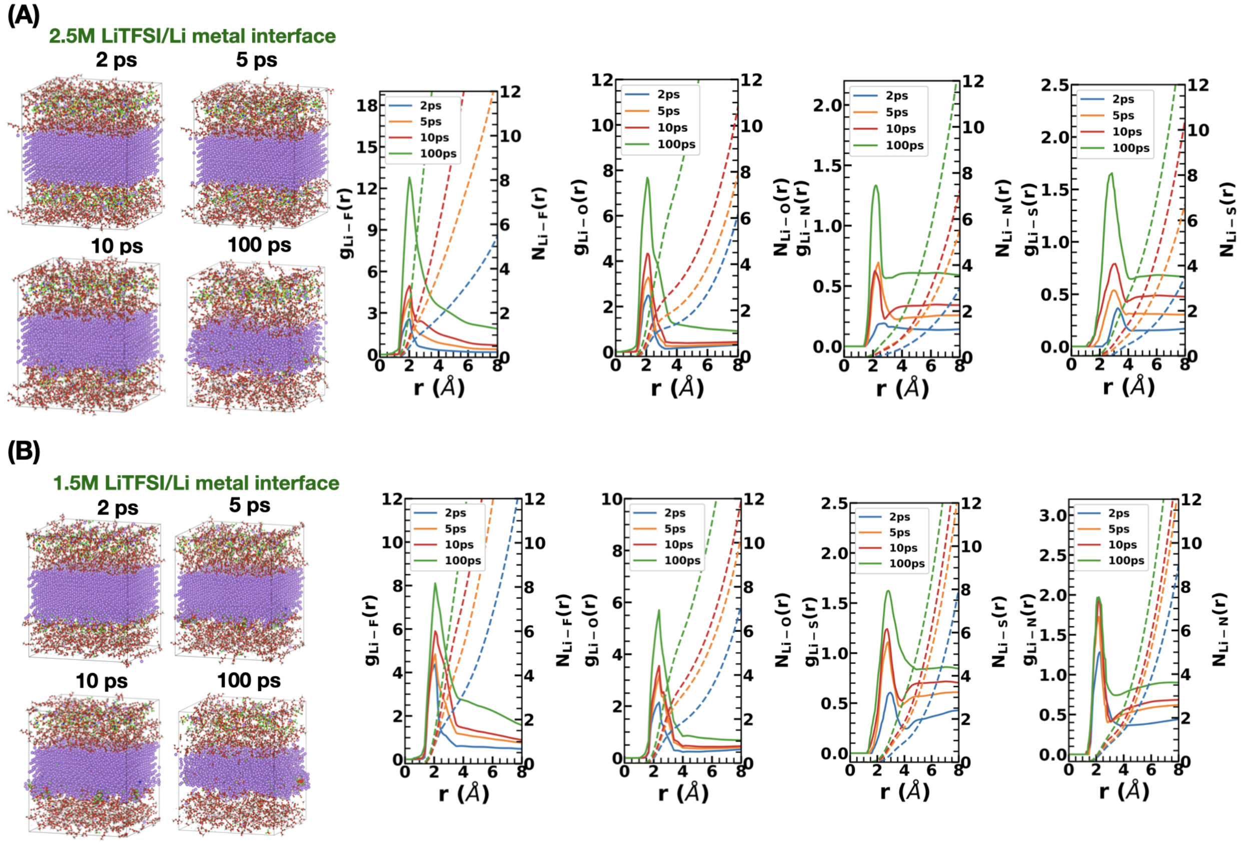


Figure S8: Time-dependent structural evolution and Li-ion solvation at the LiTFSI/Li metal interface for 2.5 M (A) and 1.5 M (B) salt concentrations.

# References


[1] L. Martínez, R. Andrade, E. G. Birgin, J. M. Martínez, Packmol: A package for building initial configurations for molecular dynamics simulations, Journal of Computational Chemistry 30 (13) (2009) 2157–2164.

[2] A. P. Thompson, H. M. Aktulga, R. Berger, D. S. Bolintineanu, W. M. Brown, P. S. Crozier, P. J. In't Veld, A. Kohlmeyer, S. G. Moore, T. D. Nguyen, et al., LAMMPS—a flexible simulation tool for particle-based materials modeling at the atomic, meso, and continuum scales, Computer Physics Communications 271 (2022) 108171.

[3] B. Doherty, X. Zhong, O. Acevedo, Virtual site opls force field for imidazolium-based ionic liquids, The Journal of Physical Chemistry B 122 (11) (2018) 2962–2974.

[4] K. Yue, B. Doherty, O. Acevedo, Comparison between ab initio molecular dynamics and opls-based force fields for ionic liquid solvent organization, The Journal of Physical Chemistry B 126 (21) (2022) 3908–3919.

[5] L. S. Dodda, I. Cabeza de Vaca, J. Tirado-Rives, W. L. Jorgensen, Ligpargen web server: an automatic opls-aa parameter generator for organic ligands, Nucleic Acids Research 45 (W1) (2017) W331–W336.

[6] J. P. Perdew, K. Burke, M. Ernzerhof, Generalized gradient approximation made simple, Physical Review Letters 77 (18) (1996) 3865.

[7] P. E. Blöchl, Projector augmented-wave method, Physical Review B 50 (24) (1994) 17953.

[8] G. Kresse, D. Joubert, From ultrasoft pseudopotentials to the projector augmented-wave method, Physical Review B 59 (3) (1999) 1758.

[9] H. J. Monkhorst, J. D. Pack, Special points for brillouin-zone integrations, Physical Review B 13 (12) (1976) 5188.

[10] L. Zhang, J. Han, H. Wang, R. Car, W. E, Deep potential molecular dynamics: a scalable model with the accuracy of quantum mechanics, Physical Review Letters 120 (14) (2018) 143001.

[11] J. Zeng, D. Zhang, D. Lu, P. Mo, Z. Li, Y. Chen, M. Rynik, L. Huang, Z. Li, S. Shi, et al., DeePMD-kit v2: A software package for deep potential models, The Journal of Chemical Physics 159 (5) (2023).

[12] S. Plimpton, Fast parallel algorithms for short-range molecular dynamics, Journal of Computational Physics 117 (1) (1995) 1–19.

[13] R. W. Hockney, J. W. Eastwood, Computer Simulation Using Particles, CRC Press, 2021.

[14] M. Deserno, C. Holm, How to mesh up ewald sums. i. a theoretical and numerical comparison of various particle mesh routines, The Journal of Chemical Physics 109 (18) (1998) 7678–7693.

[15] A. I. Jewett, D. Stelter, J. Lambert, S. M. Saladi, O. M. Roscioni, M. Ricci, L. Autin, M. Maritan, S. M. Bashusqeh, T. Keyes, et al., Moltemplate: A tool for coarse-grained modeling of complex biological matter and soft condensed matter physics, Journal of Molecular Biology 433 (11) (2021) 166841.

[16] M. Lemaalem, P. Carbonniere, Effects of solvents on $li^+$ distribution and dynamics in PVDF/LiFSI solid polymer electrolytes: An all-atom molecular dynamics simulation study, Solid State Ionics 399 (2023) 116304.
